# Supplementary material for: Strain-engineering of twist-angle in graphene/hBN superlattice devices
Source: arXiv:1810.03903 ancillary file (2018-12-04)
Supplement: Supplementary file 1 [file Supplementary_Strain-Contacts_ADeS_PAPER.pdf]

# SUPPORTING INFORMATION

## Strain-engineering of twist-angle in graphene/hBN superlattice devices

Adolfo De Sanctis,<sup>\*,†</sup> Jake Mehew,<sup>†</sup> Saad Alkhalifa,<sup>†,‡</sup> Freddie Withers,<sup>†</sup> Monica  
F. Craciun,<sup>†</sup> and Saverio Russo<sup>\*,†</sup>

<sup>†</sup>*Centre for Graphene Science, College of Engineering, Mathematics and Physical Sciences,  
University of Exeter, Exeter EX4 4QF, United Kingdom*

<sup>‡</sup>*University of Duhok, Duhok, 42001 Kurdistan Region, Iraq*

E-mail: a.de-sanctis@exeter.ac.uk; s.russo@exeter.ac.uk

# Fabrication of top- and edge-contacts

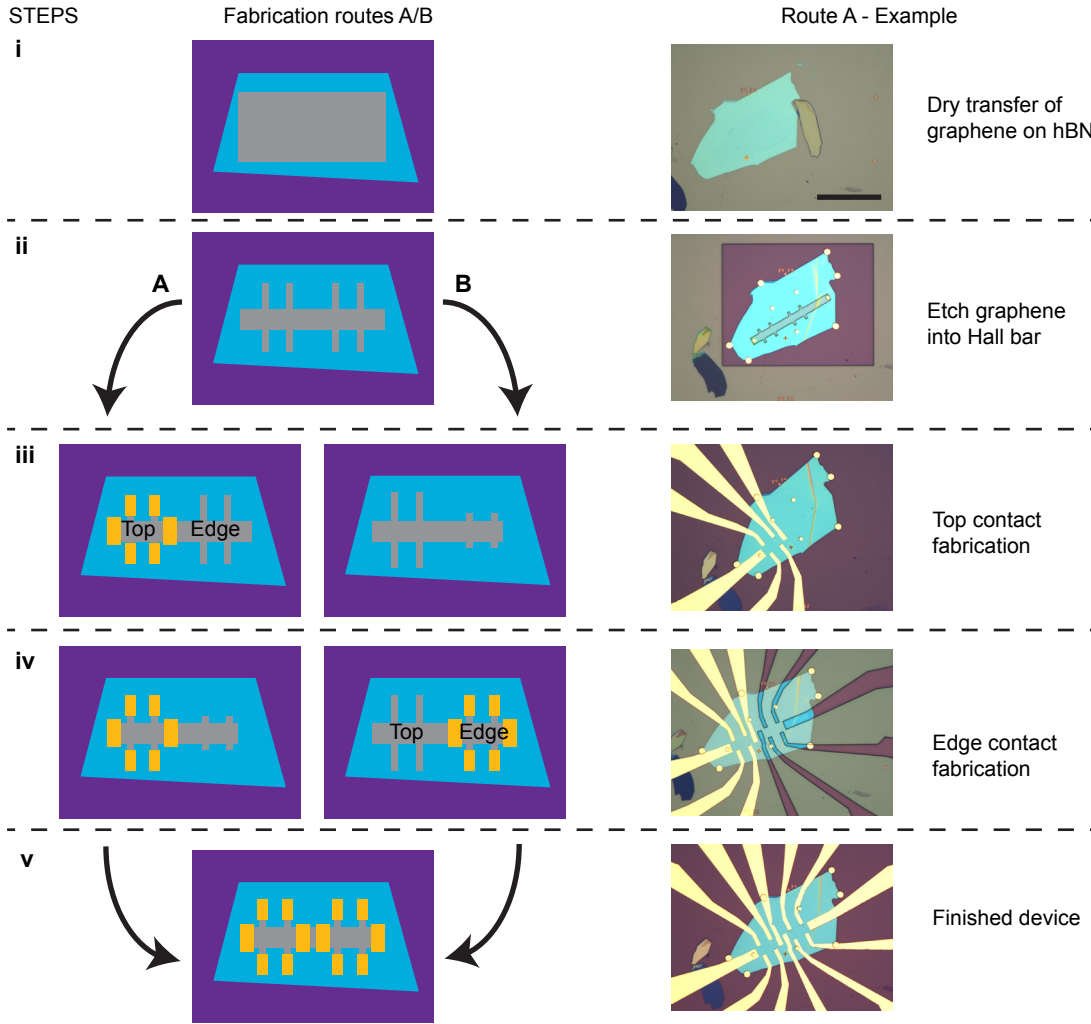

Figure S1: Schematic diagram of the fabrication steps outlined in the Methods (left) and optical micrographs of a sample device during the different steps (right).

Figure S1 outlines the lithography steps performed to fabricate a device with top- and edge-contacts. Graphene on hBN (i) is etched into Hall bar geometry using an Ar/O<sub>2</sub> plasma (ii). Deposition of metal electrodes follows one of two routes: A or B. In route A the top contacts are formed first by electron beam lithography and thermal evaporation of Cr/Au (15/60 nm) electrodes (iii). For edge contacts, the graphene/hBN heterostructure is etched in an CHF<sub>3</sub>/O<sub>2</sub> plasma (iv) before metal deposition (v). Route B differs in that the edge contacts are processed before the top contacts. The results obtained are independent of the

processing route taken.

# Vector decomposition and Raman analysis

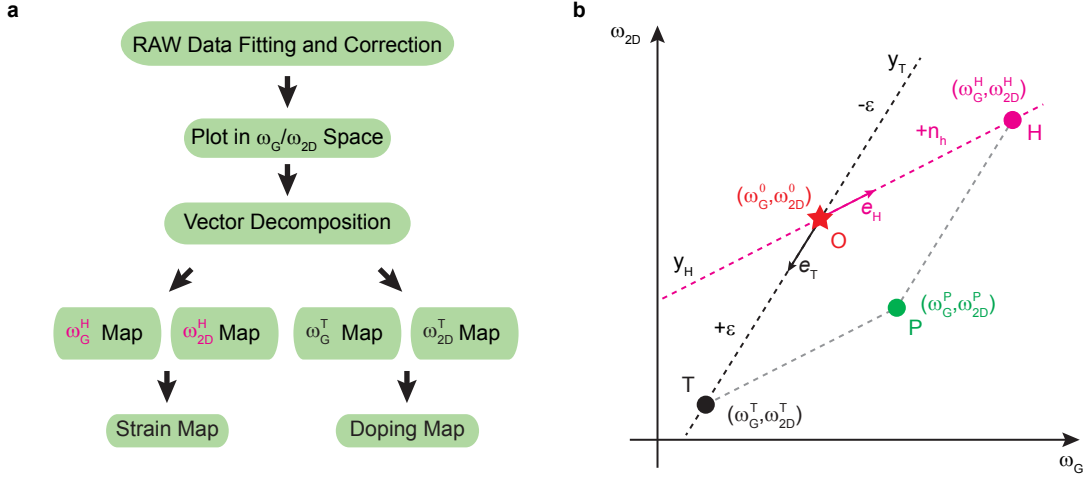

Figure S2: Vector decomposition for Raman analysis. (a) Flow diagram followed to extrapolate the strain and doping values from Raman mapping measurements. (b)  $\omega_{2D}$  vs  $\omega_G$  space diagram illustrating the vector decomposition analysis. The point  $O$  corresponds to pristine, unstrained and undoped graphene.  $y_T$  and  $y_H$  represent the iso-doping and iso-strain axes, respectively.  $P$  represents a generic measured point.  $H$  and  $T$  are the projection of  $P$  onto the two axes.  $\hat{e}_T$  and  $\hat{e}_H$  are the unit vectors of the  $y_T$  and  $y_H$  axes.

Figure S2a shows the computation flow diagram followed for extracting the strain and doping contributions to the  $\omega_G$  and  $\omega_{2D}$  peak positions.<sup>1</sup> The raw data are fit with Lorentzian peaks following an alignment step using the hBN Raman mode (which is not affected by the strain in the graphene layer). This produces the  $\omega_{2D}/\omega_G$  plot shown in figure S2b. The pristine (undoped and unstrained) graphene point is  $O$  with  $\omega_G^0 = 1581.6 \text{ cm}^{-1}$  and  $\omega_{2D}^0 = 2676.9 \text{ cm}^{-1}$ . The corresponding vector  $\vec{OP}$  for any point  $P$  in the  $\omega_G$  vs.  $\omega_{2D}$  plot can be decomposed into the strain-free  $\vec{OH}$  and charge neutral  $\vec{OT}$  direction with unit vectors  $\hat{e}_H$  for hole doping,  $\hat{e}_T$  for tensile strain and  $-\hat{e}_T$  for compressive strain. With reference to the nomenclature in figure S2b, the iso-strain and iso-doping axes (dashed lines) can be expressed as:

$$\begin{aligned} y_H &= \omega_{2D}^0 + \Delta_H (\omega_G^H - \omega_G^0) \\ y_T &= \omega_{2D}^0 + \Delta_T (\omega_G^T - \omega_G^0), \end{aligned} \tag{1}$$

whilst their equivalent passing through the point  $\mathbf{P}$  are:

$$\begin{aligned} y_{\mathbf{H}}^{\mathbf{P}} &= \omega_{2\mathbf{D}}^{\mathbf{P}} + \Delta_{\mathbf{H}} (\omega_{\mathbf{G}}^{\mathbf{T}} - \omega_{\mathbf{G}}^{\mathbf{P}}) \\ y_{\mathbf{T}}^{\mathbf{P}} &= \omega_{2\mathbf{D}}^{\mathbf{P}} + \Delta_{\mathbf{T}} (\omega_{\mathbf{G}}^{\mathbf{H}} - \omega_{\mathbf{G}}^{\mathbf{P}}), \end{aligned} \quad (2)$$

where  $\Delta_{\mathbf{H}} = (\Delta\omega_{2\mathbf{D}}/\Delta\omega_{\mathbf{G}})_{\mathbf{n}}^{\mathbf{h}} = 0.70$  and  $\Delta_{\mathbf{T}} = (\Delta\omega_{2\mathbf{D}}/\Delta\omega_{\mathbf{G}})_{\varepsilon}^{\mathbf{uni}} = 2.2$  (see also main text). Solving equation (1) and equation (2) to find their intercepts yields the coordinates of the points  $\mathbf{T}$  and  $\mathbf{H}$ , projection of the point  $\mathbf{P}$ :

$$\begin{aligned} \omega_{\mathbf{G}}^{\mathbf{H}} &= \frac{\omega_{2\mathbf{D}}^{\mathbf{P}} - \omega_{2\mathbf{D}}^0 + \Delta_{\mathbf{H}}\omega_{\mathbf{G}}^0 - \Delta_{\mathbf{T}}\omega_{\mathbf{G}}^{\mathbf{P}}}{\Delta_{\mathbf{H}} - \Delta_{\mathbf{T}}} \\ \omega_{2\mathbf{D}}^{\mathbf{H}} &= \omega_{2\mathbf{D}}^{\mathbf{P}} + \Delta_{\mathbf{T}}(\omega_{\mathbf{G}}^{\mathbf{H}} - \omega_{\mathbf{G}}^{\mathbf{P}}) \\ \omega_{\mathbf{G}}^{\mathbf{T}} &= \frac{\omega_{2\mathbf{D}}^{\mathbf{P}} - \omega_{2\mathbf{D}}^0 + \Delta_{\mathbf{T}}\omega_{\mathbf{G}}^0 - \Delta_{\mathbf{H}}\omega_{\mathbf{G}}^{\mathbf{P}}}{\Delta_{\mathbf{T}} - \Delta_{\mathbf{H}}} \\ \omega_{2\mathbf{D}}^{\mathbf{T}} &= \omega_{2\mathbf{D}}^{\mathbf{P}} + \Delta_{\mathbf{H}}(\omega_{\mathbf{G}}^{\mathbf{T}} - \omega_{\mathbf{G}}^{\mathbf{P}}). \end{aligned} \quad (3)$$

Finally, the doping and strain values can be calculated using:

$$\begin{aligned} \Delta\varepsilon &= \frac{\Delta\omega_{\mathbf{G}}^{\mathbf{T}}}{-23.5} \% \\ \Delta n &= \frac{\Delta\omega_{\mathbf{G}}^{\mathbf{H}}}{-13.1} 10^{13} \text{ cm}^{-2}, \end{aligned} \quad (4)$$

with the conversion value for strain ( $-23.5 \text{ cm}^{-1}/\%$ ) and doping ( $-13.1 \text{ cm}^{-1}/10^{13} \text{ cm}^{-2}$ ) taken from literature.<sup>2,3</sup>

To confirm that the procedure just outlined was able to resolve the necessary strain and doping distributions in graphene/hBN devices, we performed the analysis of a single-layer graphene flake deposited both on hBN and on  $\text{SiO}_2$ , as shown in the optical micrograph in figure S3a. The raw data after the Lorentzian fitting are also shown in figure S3a. Figure S3b shows the  $\omega_{\mathbf{G}}/\omega_{2\mathbf{D}}$  space diagram for the two regions separated (hBN and  $\text{SiO}_2$ ). We notice the upshift of the points extracted from the hBN region with respect to the ones on the  $\text{SiO}_2$ . Using equation (3) the points are projected on the corresponding iso-strain and iso-doping axes (figure S3b, inset) and four maps can be extracted, as shown in figure S3c. Using

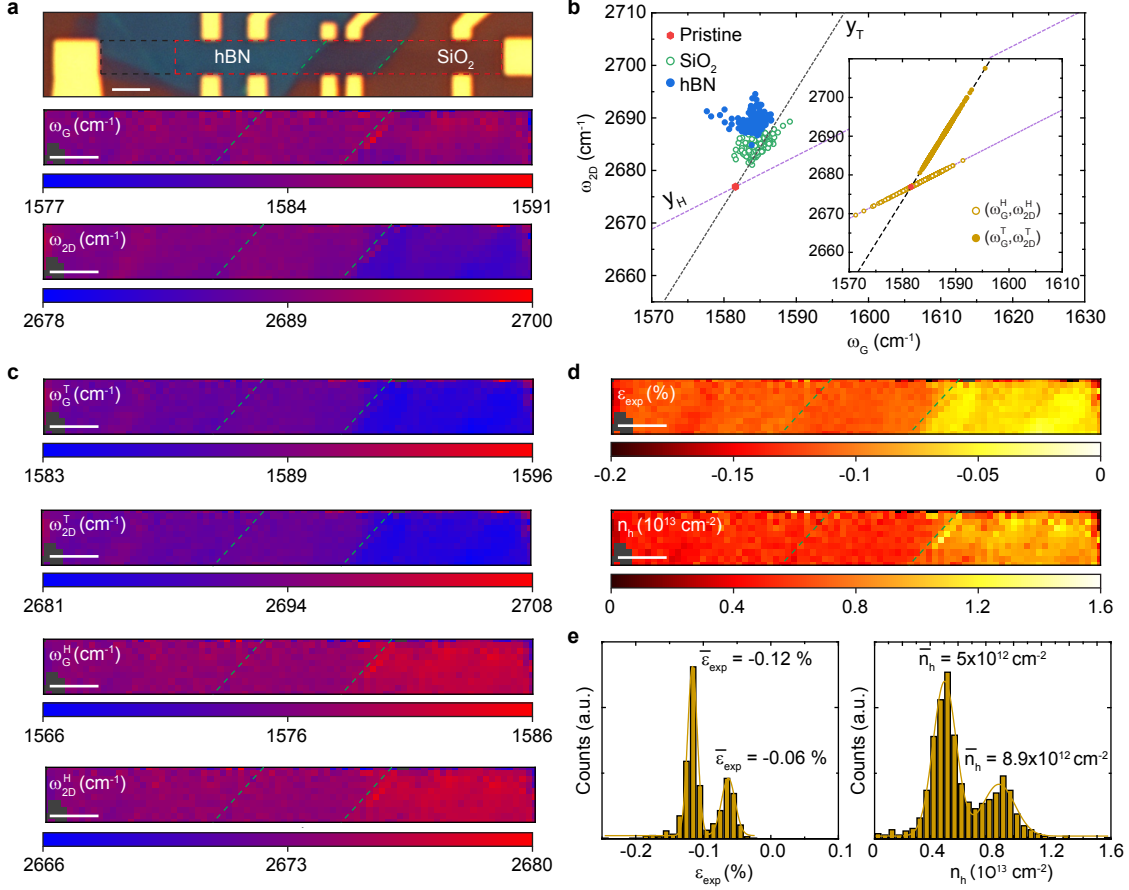

Figure S3: Calibration of Raman setup and vector analysis. (a) Optical micrograph (top) and raw data  $\omega_G/\omega_{2D}$  maps (bottom) of a graphene flake covering both hBN and SiO<sub>2</sub>. (b)  $\omega_G/\omega_{2D}$  space diagram from the maps in panel (a) for the hBN (filled circles) and SiO<sub>2</sub> (open circles) regions. Inset: projected experimental points after vector decomposition. (c) Intermediate maps representing the distribution of the iso-strain and iso-doping points after applying 3. (d) Extrapolated strain and doping maps from the data in panel (c). (e) Statistical distributions extrapolated from the maps in panel (d). Scale-bars are 2  $\mu$ m.

equation (4) the strain and doping maps can be computed, as shown in figure S3d. Statistical analysis on these maps reveals distributions characterised by two peaks (figure S3e). The strain distribution has peaks at  $\bar{\varepsilon}_{\text{exp}} = -0.12\%$  and  $\bar{\varepsilon}_{\text{exp}} = -0.06\%$ , of which the former is related to the graphene/hBN region and the latter to the graphene/SiO<sub>2</sub> region. Similarly the doping distribution shows peaks at  $\bar{n}_{\text{h}} = 5 \cdot 10^{12} \text{ cm}^{-2}$  (hBN) and  $\bar{n}_{\text{h}} = 8.9 \cdot 10^{12} \text{ cm}^{-2}$  (SiO<sub>2</sub>), which is consistent with previous reports by other authors.<sup>1,4,5</sup>

## Supplementary data: Raman mapping and other devices

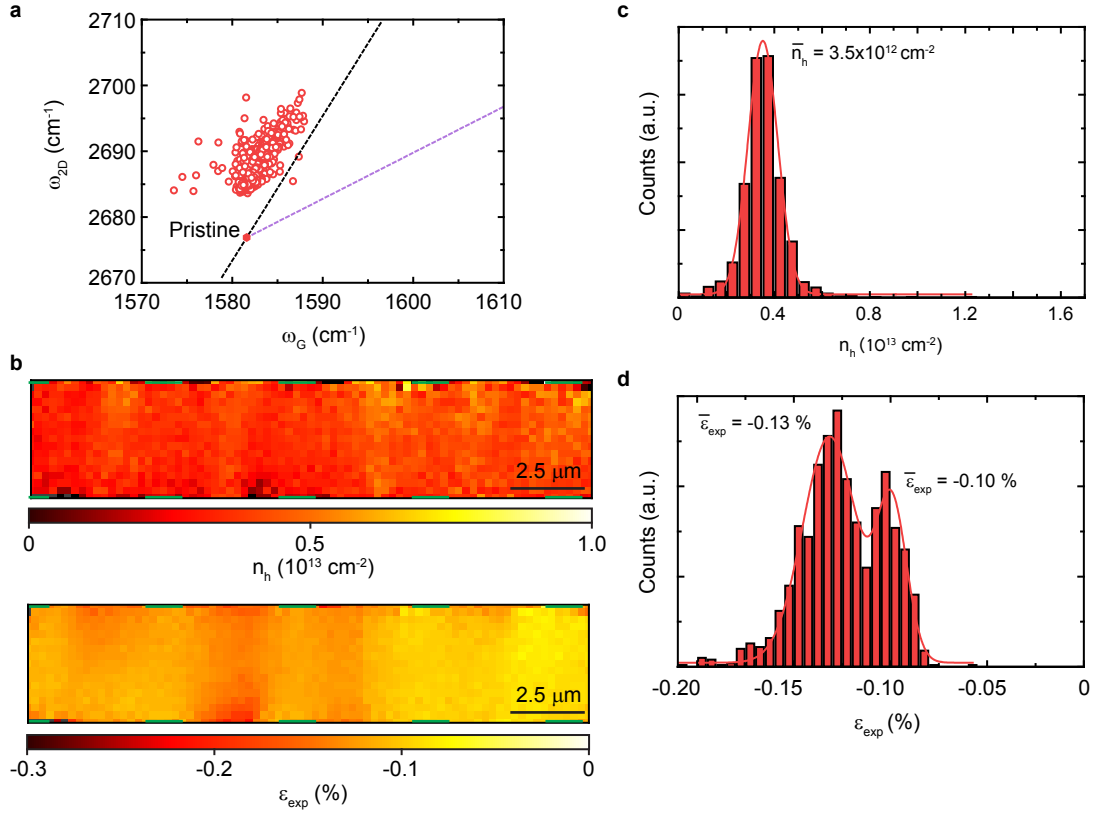

Figure S4: Raman analysis of a top-contacted device. (a)  $\omega_G/\omega_{2D}$  space diagram for a top-contacted device with multiple contacts. (b) Doping (top) and strain (bottom) maps of the device. Top-contacts positions are shown by green solid lines. (c) and (d), Statistical distributions extrapolated from the maps in panel (b).

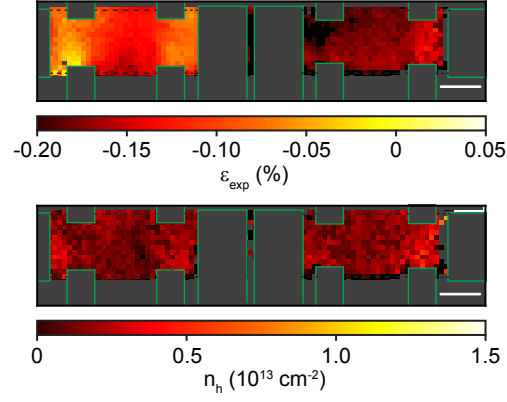

Figure S5: Experimentally determined strain (top,  $\varepsilon_{\text{exp}}$ ) and doping (bottom,  $n_h$ ) maps across the device in Figure 1 main text after thermal annealing. Negative sign indicates compressive strain. Scalebars are  $2 \mu\text{m}$ .

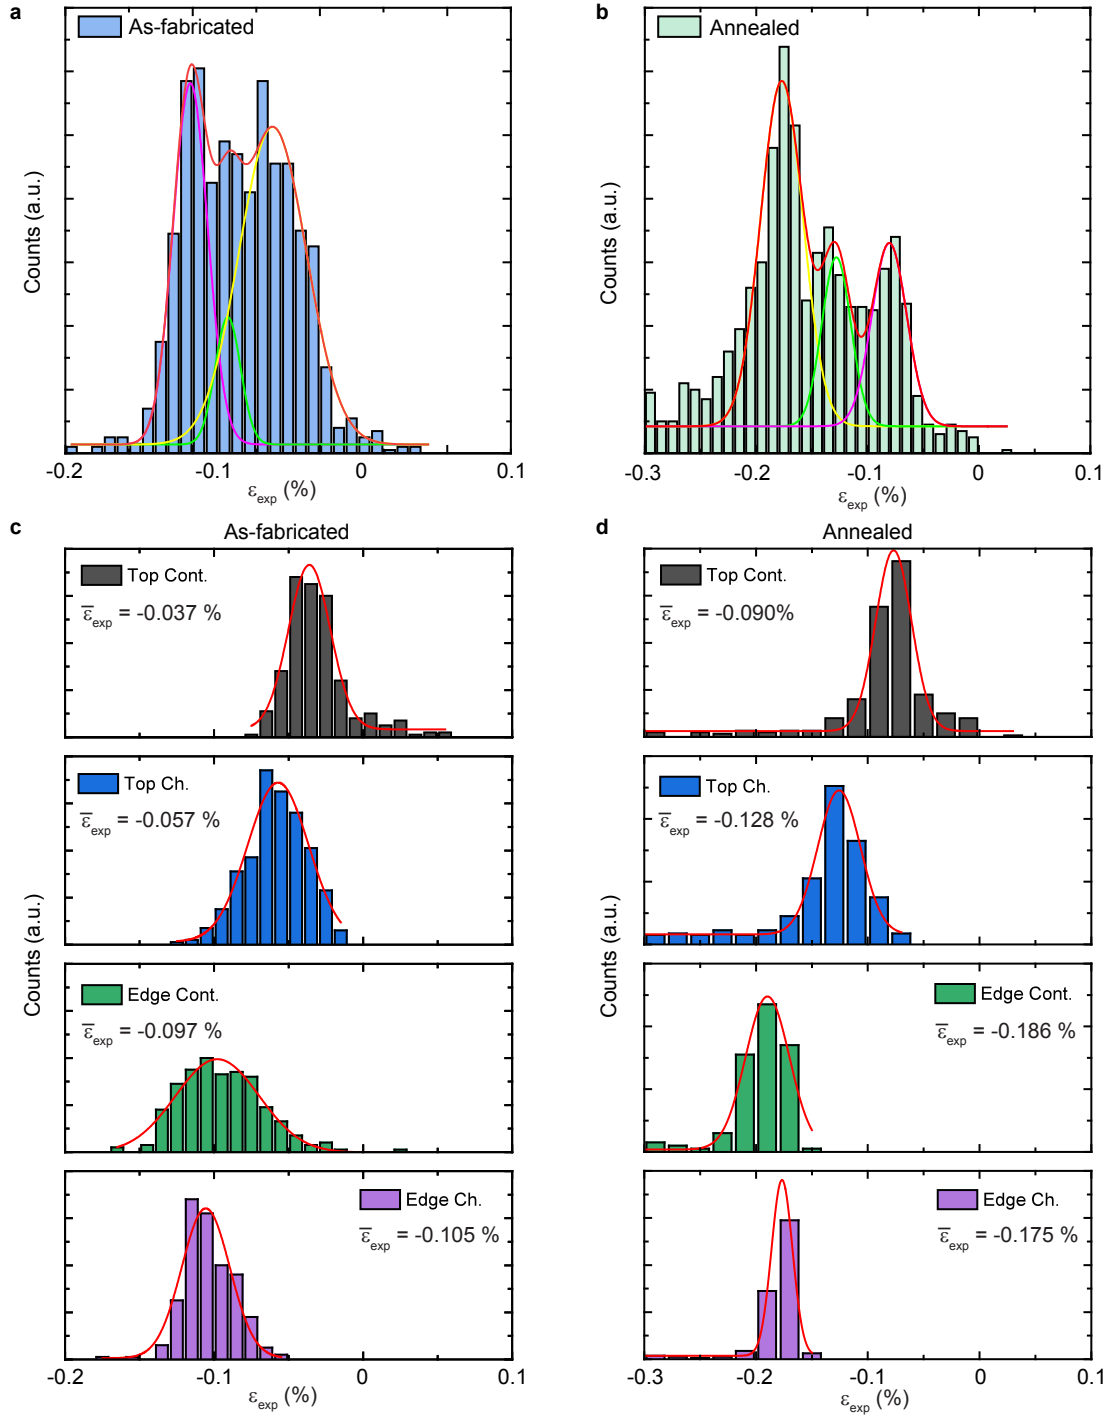

Figure S6: Statistical analysis of strain. (a) Detailed Gaussian fit of the data shown in Figure 3b (main text) before and (b) after annealing. (c) Statistical analysis and Gaussian fit of the data from Figure 3b (main text) extrapolated from four different regions in the map shown in Figure 1 (main text). (d) Same analysis performed on the data from the map in Figure S5. It is evident that the three Gaussian curves in the combined fits (a) and (b)) arise from three different regions.

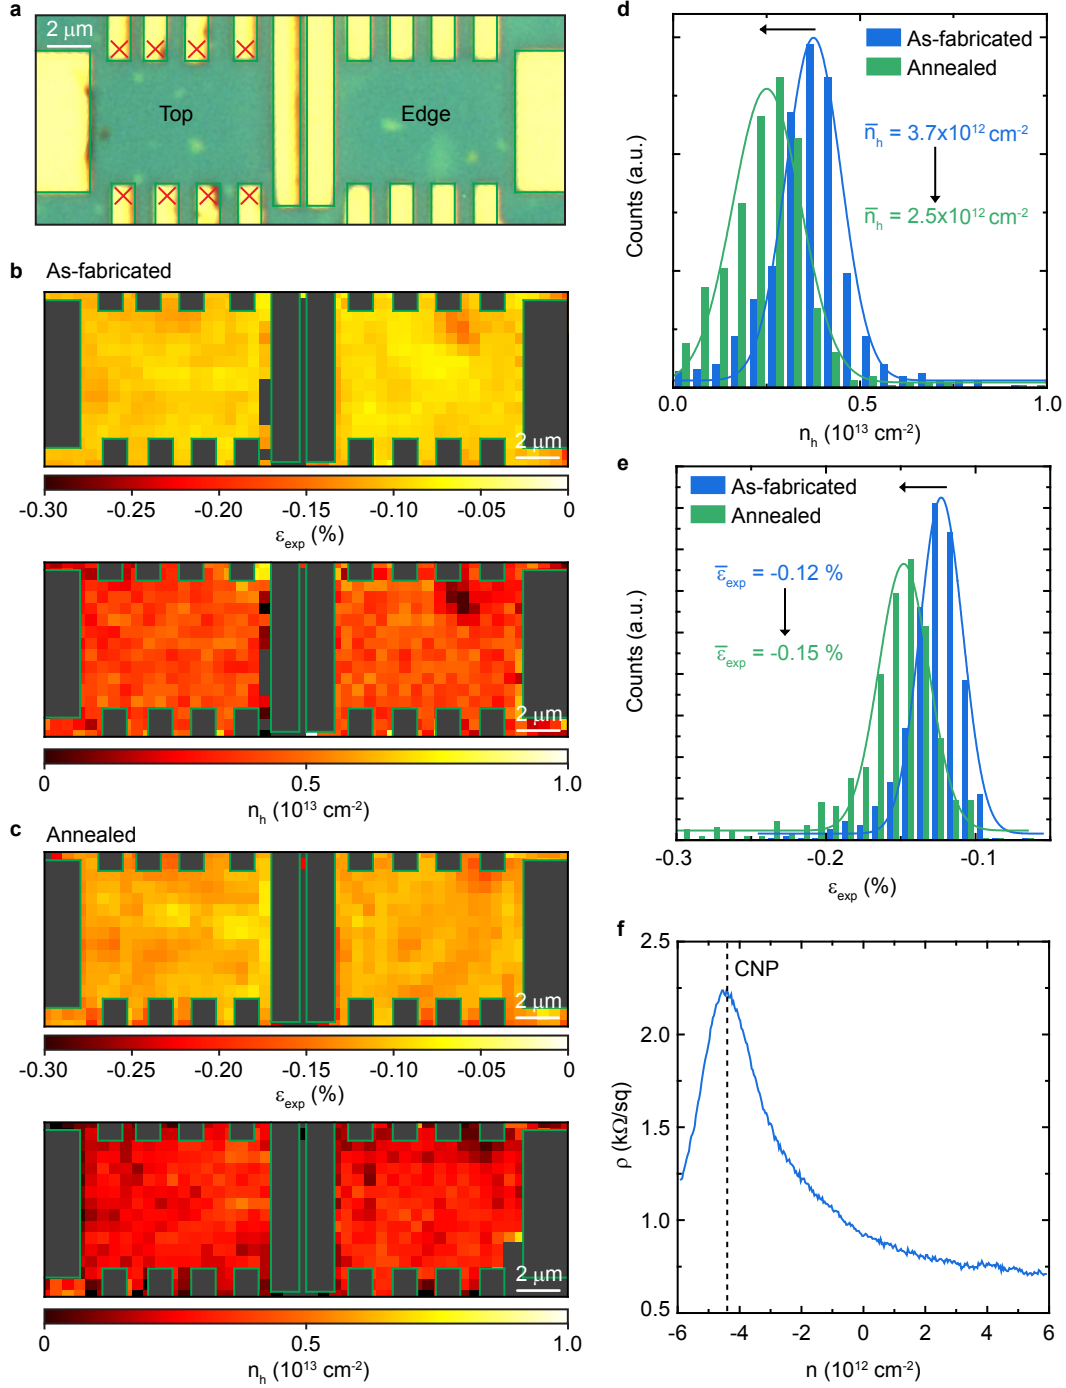

Figure S7: Analysis of a broken device. (a) Optical micrograph of a device in which the top-contacts have no electrical connection to the graphene. (b) and (c), Strain and doping maps of the device before and after thermal annealing. (d) and (e), statistical distributions extrapolated from the maps in panels (b) and (c). (f) Resistivity measured in the edge-contacted region as a function of charge density. The CNP appears at  $n \sim -4 \cdot 10^{12}\ \text{cm}^{-2}$ , in line with the results from Raman analysis shown in panel (d).

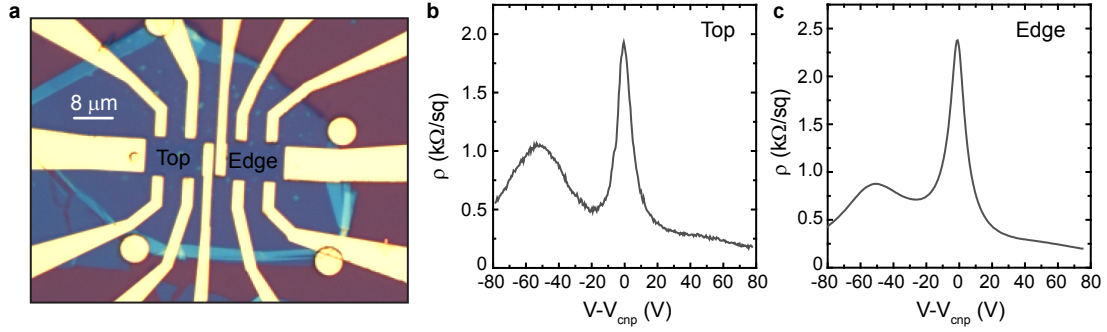

Figure S8: G/hBN superlattices example. (a) Optical micrograph of another device fabricated following the same procedure outlined in the methods. Scale-bar is  $8\ \mu\text{m}$ . (b), (c) Resistivity as a function of gate voltage for the top- and edge-contact, respectively. The alignment of the graphene to the hBN is evident from the appearance of the satellite peak.

## References

- (1) Lee, J. E.; Ahn, G.; Shim, J.; Lee, Y. S.; Ryu, S. *Nature Communications* **2012**, *3*, 1024.
- (2) Yoon, D.; Son, Y.-W.; Cheong, H. *Phys. Rev. Lett.* **2011**, *106*, 155502.
- (3) Das, A.; Pisana, S.; Chakraborty, B.; Piscanec, S.; Saha, S. K.; Waghmare, U. V.; Novoselov, K. S.; Krishnamurthy, H. R.; Geim, A. K.; Ferrari, A. C.; Sood, A. K. *Nature Nanotechnology* **2008**, *3*, 210.
- (4) Neumann, C.; Reichardt, S.; Venezuela, P.; Drögeler, M.; Banszerus, L.; Schmitz, M.; Watanabe, K.; Taniguchi, T.; Mauri, F.; Beschoten, B.; Rotkin, S. V.; Stampfer, C. *Nature Communications* **2015**, *6*, 8429.
- (5) Engels, S.; Terrés, B.; Klein, F.; Reichardt, S.; Goldsche, M.; Kuhlen, S.; Watanabe, K.; Taniguchi, T.; Stampfer, C. *Physica Status Solidi (b)* **2014**, *251*, 2545–2550.
